# Supplementary material for: Switching of an antiferromagnet controlled by spin canting in a laser-induced hidden phase
Source: arXiv:2504.12929 ancillary file (2025-12-16)
Supplement: Supplementary file 1 [file Supplementary_material.pdf]

# Switching of an antiferromagnet controlled by spin canting in a laser-induced hidden phase: Supplementary material

A. V. Kuzikova,[1,*] N. A. Liubachko,[2] S. N. Barilo,[2] A. V. Sadovnikov,[3] R. V. Pisarev,[1] and A. M. Kalashnikova[1]

[1]*Ioffe Institute, 194021 St. Petersburg, Russia*

[2]*Scientific-Practical Materials Research Centre, NAS of Belarus, 220072 Minsk, Belarus*

[3]*Laboratory "Magnetic Metamaterials", Saratov State University, 410001 Saratov, Russia*

(Dated: April 17, 2025)

## I. MAGNETO-OPTICAL HYSTERESIS LOOPS

In order to characterize magnetic anisotropy of the sample at equilibrium, probe polarization rotation $\theta_S$ was measured at different temperatures $T_0$ as a function of an external magnetic field without pump excitation $\mu_0 H$ (Fig.1) in the experimental geometry shown in Fig. 2(a). Probe angle of incidence of 45° ensures that the polarization rotation is sensitive to the out-of-plane magnetization through the polar magneto-optical Kerr effect (MOKE) at $T_0 < T_{\mathrm{SR}}$, and to the in-plane magnetization through the longitudinal MOKE at $T_0 > T_{\mathrm{SR}}$. The shape of the loop at $T_0 < T_{SR}$ indicates that magnetization is directed along the $a$-axis, and the field strength is insufficient to deviate the magnetization from this axis.

* anna.kuzikova@mail.ioffe.ru

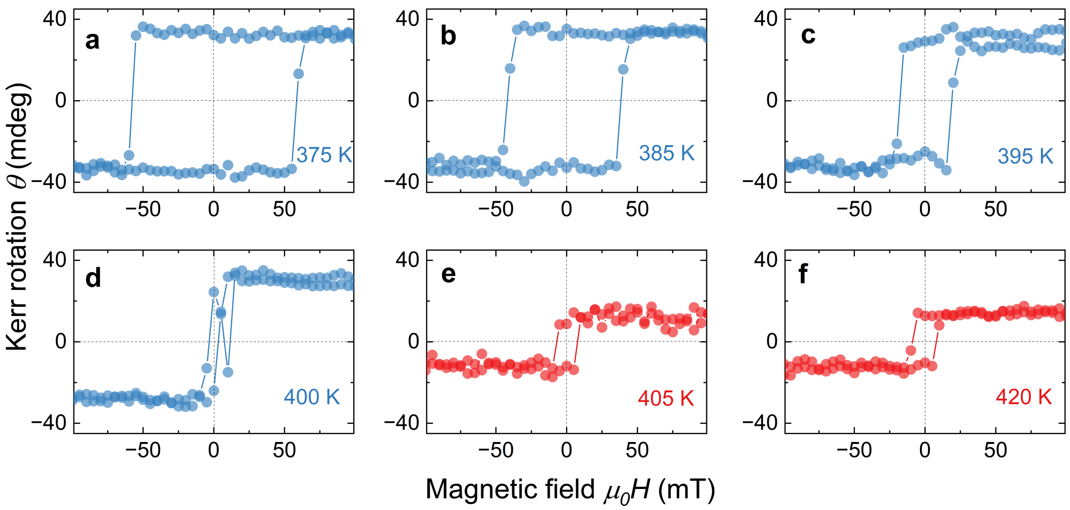


FIG. 1. Equilibrium magneto-optical hysteresis loops measured at various temperatures $T_0$ without pump excitation.

## II. EXPERIMENTAL

We employed a femtosecond two-color magneto-optical pump-probe technique to study temporal evolution of magnetization following laser excitation [Fig. 2(a)]. Pump and probe pulses with duration 170 fs were emitted by $Yb^{3+}$:$KGd(WO_4)_2$ regenerative amplifier at a repetition rate of 5 kHz. Incident pump pulses with a central wavelength of 1030 nm were focused normally to the sample surface into a spot with a diameter of 45 µm. Probe pulses with a central wavelength of 515 nm were focused into the spot with a diameter of 30 µm at an incidence angle of 45°. The external magnetic field $\mu_0 H = 40 - 240$ mT was applied in the direction close to the *c*-axis. The pump fluence $F$ was varied in the range 0.2–0.6 J·cm$^{-2}$, and the probe fluence was around 4 mJ·cm$^{-2}$. Laser-induced change of magneto-optical rotation of the probe polarization $\Delta\theta$ was measured as a function of pump-probe time delay $t$. To extract the field-sign dependent contribution, the signals were evaluated as

$$\Delta\theta(t) = 0.5\left[\Delta\theta(H_+;t) - \Delta\theta(H_-;t)\right]. \quad (1)$$

An example of the time delay dependences measured at negative and positive fields and their difference is shown in Fig. 2(b,c).

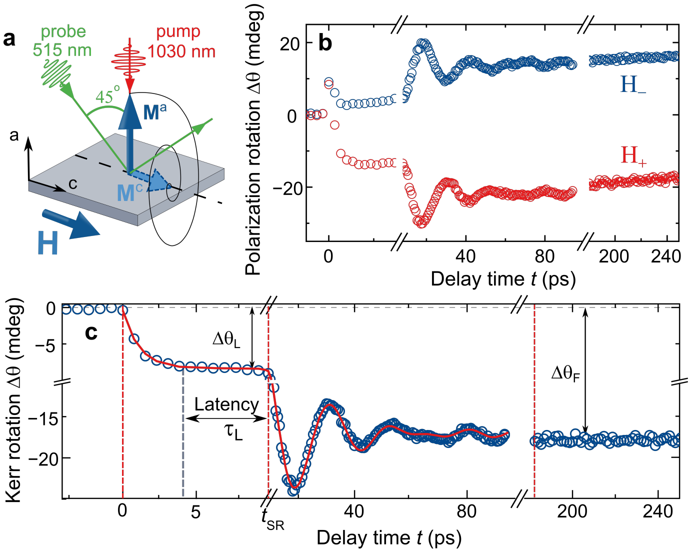


FIG. 2. (a) Experimental geometry for the magneto-optical detection of the equilibrium and laser-induced SR transition. (b) Laser-induced probe polarization rotation $\Delta\theta$ as a function of time delay $t$ measured in the magnetic field $\mu_0 H = \pm 200$ mT at $T_0$= 385 K and $F = 0.5$ J·cm$^{-2}$. (c) The corresponding field-sign dependent contribution to the signal $\Delta\theta(t)$ according to Eq. (1). Line shows the fit according to Eq. (2).

## III. FIT OF TRANSIENT MOKE SIGNALS

The dependence of the probe polarization rotation $\Delta\theta$ on the time delay between the pump and probe pulses has a non-trivial behavior with a rapid decrease within a few picoseconds after the excitation, followed by a latency $\tau_L$ during which the signal remains constant at the value $\Delta\theta = \Delta\theta_L$ [Fig.2(c)]. After the latency, at $t = t_{SR}$ pronounced decaying oscillations start resulting in a signal settling at a final level $\Delta\theta = \Delta\theta_F$. To provide quantitative description of this behavior, we fitted the time-traces using a piecewise function:

$$\Delta\theta(t) = \begin{cases} \Delta\theta_L \left[\exp\left(-\frac{t}{\tau_1}\right) - 1\right], & \text{for } t < t_{SR}; \\ \Delta\theta_F \left[\exp\left(-\frac{t-t_{SR}}{\tau_2}\right) - 1\right] + \sum_{i=1,2} \Theta_i \exp\left(\frac{-t}{\tau_{oi}}\right) \cos\left[2\pi f_i t + \phi_i\right], & \text{for } t > t_{SR}, \end{cases} \quad (2)$$

where $\Delta\theta_{L,F}$ are the signals during the latency and at the final state; $\tau_{1,2}$ - characteristics times of two exponential functions. Oscillating signal are characterized by their amplitudes $\Theta_i$, decay times $\tau_{oi}$, frequencies $f_i$, and initial phases $\phi_i$.

## IV. ANALYSIS OF MAGNETIC ENERGY AND CALCULATION OF FMR FREQUENCY

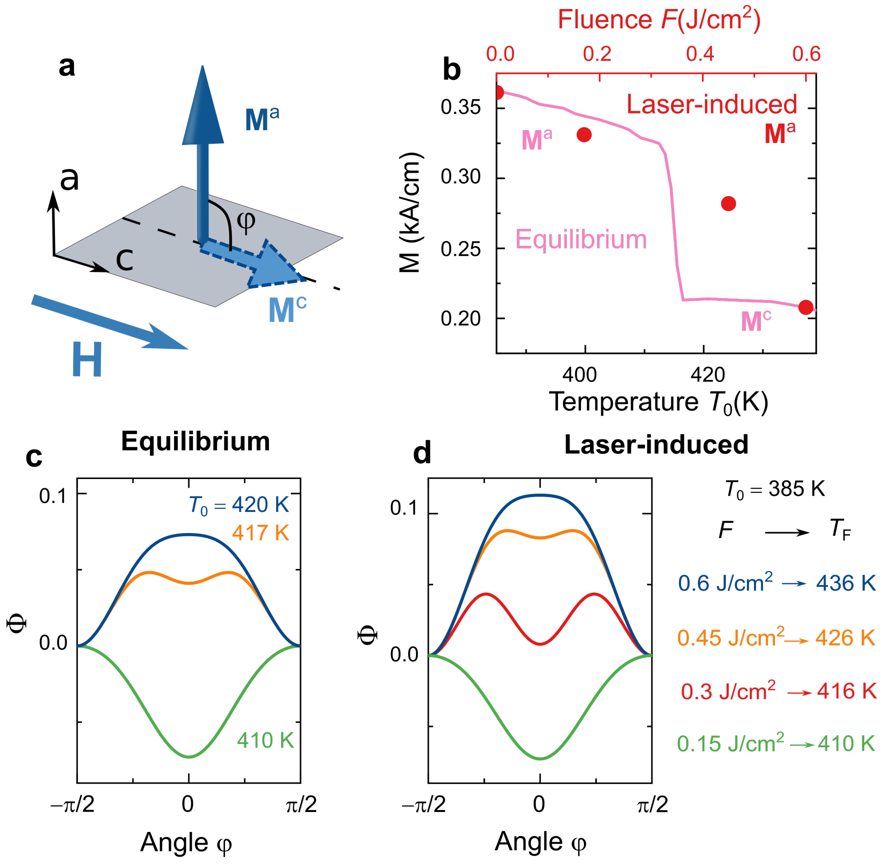


FIG. 3. (a) Schematics of the magnetization orientations at the $\Gamma_2$ ($M^a$) and the $\Gamma_4$ ($M^c$) phases. (b) Line: magnetization $M^a$ and $M^c$ as a function of temperature $T_0$ at equilibrium, as adapted from Ref. [1]. Symbols: magnetization $M^a$ after laser excitation as a function of fluence $F$ (symbols), as calculated from $\theta_L$ (see text). (c) Calculated energy profile $\Phi$ vs. the angle between the magnetization and the $a$-axis. at equilibrium at $T_0$ = 410 (green), 417 (blue), 420 K (orange). (d) Calculated energy profile $\Phi(\phi)$ as a result of laser excitation at fixed $T_0$ = 385 K and $F$ = 0.15 (green), 0.3 (red), 0.45 (orange), 0.6 J·cm$^{-2}$ (blue). Corresponding effective heating temperatures are $T_{\mathrm{F}}$ = 410 (green), 416 (red), 426 (orange), 436 K (blue).

### A. Magnetic part of the free energy

For theoretical description of a magnetic state of $Fe_3BO_6$, an expansion of the thermodynamic potential for the two subsystem antiferromagnet with the *Pnma* group is used [2]:

$$\Phi = \frac{E}{2}m^2 - d_a m_a l_c + d_c m_c l_a + \frac{a_1}{2}l_c^2 + \frac{c_1}{2}l_a^2 + \frac{a_2}{4}l_c^4 + \frac{c_2}{4}l_a^4 + \frac{f}{2}l_c^2 l_a^2 - mH. \tag{3}$$

where $m = (M_1 + M_2)/M_0$, and $l = (M_1 - M_2)/M_0$, are the ferromagnetic and antiferromagnetic vectors, respectively. $M_1$ and $M_2$ are the magnetic moments of the sublattices, $M_0$ is their magnitude at the given temperature. $E/2$ is effective exchange parameter, $d_a$, $d_c$ are effective parameters of the DMI, $a_1$, $c_1$, $a_2$, $c_2$, $f$ are the bilinear and biquadratic magnetocrystalline anisotropy parameters. $H$ is the external magnetic field.

To describe the connection between the phase transition conditions and the DMI parameters, we use the formalism introduced in [3]. The anisotropic part of the thermodynamic potential can be transformed into

$$\Phi = K_1 \cos^2 \varphi + K_2 \cos^4 \varphi. \tag{4}$$

where $K_1$, $K_2$ are the effective anisotropy constant, $\varphi$ is an angle between the magnetization $m$ and the $a$-axis, as shown in Fig. 3(a). Taking into account Eq. (3), the dependence of the effective anisotropy constants $K_1$, $K_2$ in Eq. (4) on the DMI parameters and the magnetization can be obtained:

$$K_1 = d_c m - d_a m + a_2 \cdot m^2 - \frac{a_1}{2} + \frac{c_1}{2} - \frac{a_2}{2} + \frac{f}{2};$$
$$K_2 = -\frac{a_2}{2}m^2 - \frac{c_2}{2}m^2 + \frac{a_2}{4} + \frac{c_2}{4} - \frac{f}{2}, \tag{5}$$

where the conditions $l^2 + m^2 = 1$ and $m \ll 1$ were used. The combinations $A_1 = -a_1/2 + c_1/2 - a_2/2 + f/2$ and $A_2 = a_2/4 + c_2/4 - f/2$ was used in main text [Eq. 3].

### B. SR transition at equilibrium

In Fig. 3(c,d) energy profiles for the equilibrium and the laser-induced cases are shown. The main difference between these two cases is in the magnitude and orientation of the magnetization $m$, which enters the effective anisotropy constants [Eq. (5)]. For the equilibrium

case, the magnetization $m$ at $T < T_{\rm SR}$ is along the $a$-axis and is proportional to $d_a(E-c_2)^{-1}$. Above $T_{\rm SR}$ it is aligned aligned along the c-axis and is proportional to $d_c(E-a_2)^{-1}$. The value of magnetization $m$ has a discontinuity of $\approx 35\%$ at $T_{\rm SR}$[Fig. 3(b)]. Using values of $M^a$, $M^c$ from [1], the equilibrium energy profiles at various temperatures are calculated [Fig. 3(c)]. Obtained narrow temperature range where the energy profile possesses local and global minima is narrow, in agreement with the properties of $Fe_3BO_6$.

### C. SR transition under laser excitation

In the case of a laser-induced SR transition, magnetization $m$ remains along the $a$-axis upto $t_{\rm SR}$, with its value changing continuously as a function of fluence. Thus, the discontinuity in the magnetization value characteristic for the equilibrium case is absent. For each pump fluence, we used $\theta_S + \Delta\theta_L$ to estimate the magnetization value $M^a$ after the excitation, as shown in Fig. 3(b). These values were substituted into the Eq. (5), and the energy profiles were calculated. Corresponding final temperatures $T_{\rm F}$ were taken from BLS data [Fig. 3(f) in main text]. In Fig. 3(d), the laser-induced energy profiles for several $F$ and corresponding effective heating temperatures $T_{\rm F}$ are plotted. One sees that the domain of coexistence of the $\Gamma_2$ and $\Gamma_4$ phases is, indeed, effectively expanded. As discussed in the main text, the state with only one minimum at $\phi = \pi/2$ emerges at $d_a \approx d_c$ with a correction for a difference in the anisotropy parameters $a_2$ and $c_2$.

### D. FMR frequency in the $\Gamma_4$ phase

To calculate the FMR frequency in the $\Gamma_4$ phase, we note that the external magnetic field $H$ is applied along the $c$-axis being the easy axis in this phase. Then the frequency can be calculated using the expression [4]:

$$f = \gamma(H + H_{\rm A}), \tag{6}$$

where $\gamma$ =28 GHz·T$^{-1}$ is the gyromagnetic ratio, and $H_{\rm A} = 2K_1(M_S^c)^{-1}$ is the effective anisotropy field. For calculations, $M_S^c = 1900$ A·m$^{-1}$ was taken from [1], $K_1 = 1.6\cdot 10^3$ J· m$^{-3}$ was obtained from the FMR data at $T_0 = 430$ K in zero external field [5]. Calculated field dependence of the equilibrium FMR frequency is shown in Fig. 2(c) in the main manuscript.

## V. TEMPERATURE AND FLUENCE DEPENDENCES

Joint analysis of the evolution of the signals and their parameters at the initial temperature $T_0$ and fixed laser fluence $F = 0.5$ J/cm$^2$ is performed to further confirm that SR transition is observed and to evaluate the role of laser-induced heating.

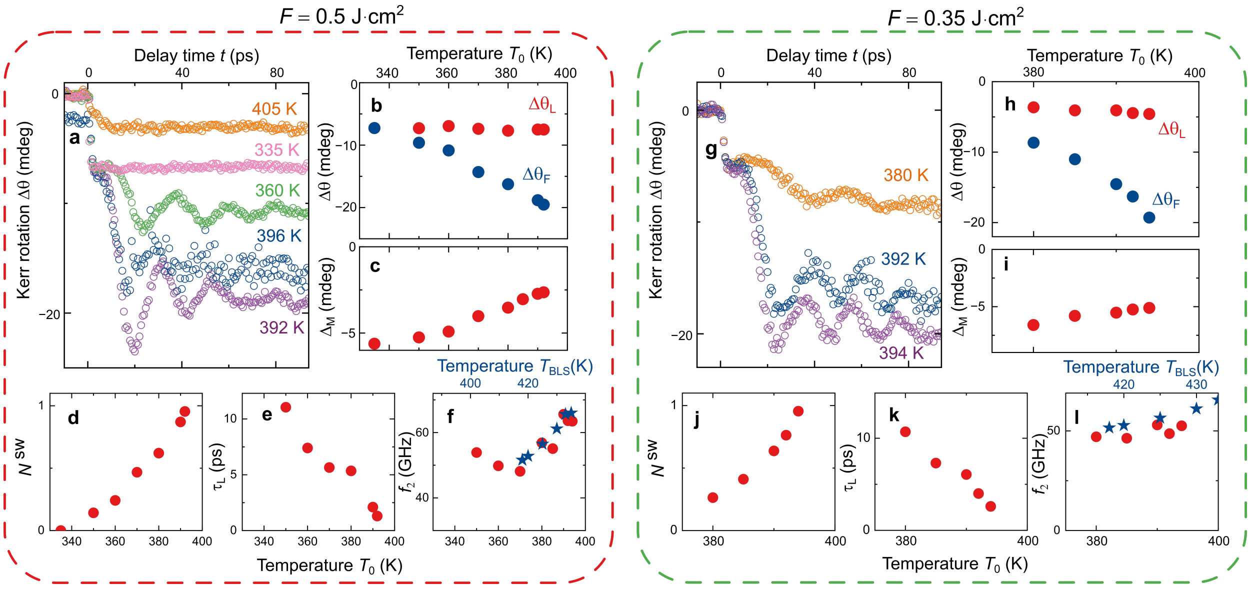


FIG. 4. Pump-probe signals $\Delta\theta(t)$ (symbols) measured at (a) $F = 0.5$ J/cm$^2$ and (g) $F = 0.35$ J/cm$^2$ at various initial temperatures at $\mu_0 H = 200$ mT. (b, h) Temperature dependence of $\Delta\theta_L$ (red symbols) and $\Delta\theta_F$ at $t > 100$ ps (blue symbols). Temperature dependence of (c, i) the magnetization mismatch parameter $\Delta_M$, (d, j) the switched fraction $N^{SW}$, and (e, k) the latency $\tau_L$ for fixed $F = 0.5$ J/cm$^2$ and $F = 0.35$ J/cm$^2$. (f, l) Collated dependences of the precession frequency $f_2$ on the initial temperature (circles), and of the qFMR frequency on the temperature $T_{BLS}$ obtained from BLS data (stars).

Fig. 4(a) shows the pump-probe signals measured at various initial temperature at fixed fluence $F = 0.5$ J·cm$^{-2}$. The precession is observed only in the range of 335 K$< T_0 < T_{SR}$, when the sample is at the $\Gamma_2$ phase initially and the fluence is sufficient to induce the SR transition. This confirms the threshold nature of the laser-induced phase transition that triggers the magnetization precession.

Importantly, when the initial temperature $T_0$ is close to $T_{SR}$, additional changes appear in the Kerr rotation $\Delta\theta$. As can be seen in Fig. 4(a), for these temperatures at negative time delays, the signal $\Delta\theta$ is not equal to zero. At $T_0 > T_{SR}$ the signal $\Delta\theta$ at $t < 0$ is zero again.

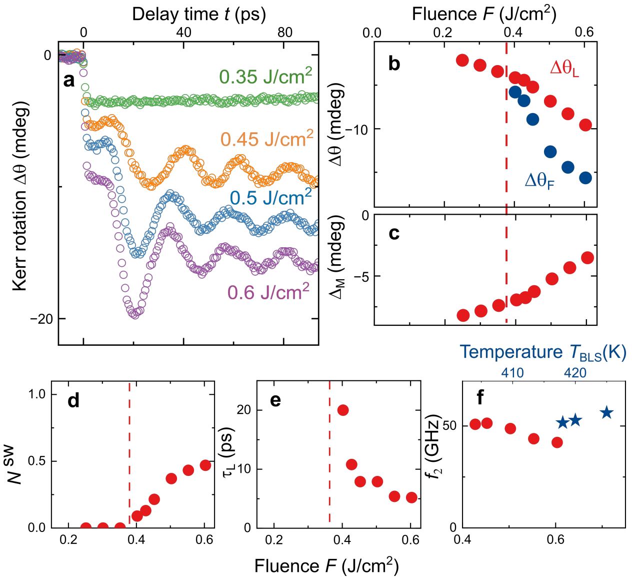


FIG. 5. (a) Pump-probe signals $\Delta\theta(t)$ (symbols) measured at $\mu_0 H$ =200 mT and $T_0$ = 365 K at various fluence. (b) Fluence dependence of $\Delta\theta_{\mathrm{L}}$ during the latency (red symbols) and the $\Delta\theta_{\mathrm{F}}$ at $t > 100$ ps (blue symbols). (c-e) Fluence dependence of (c) the magnetization mismatch parameter $\Delta_{\mathrm{M}}$, (d) the fraction $N^{\mathrm{SW}}$ of the material switched to the $\Gamma_4$ phase, and (e) the latency $\tau_{\mathrm{L}}$. (f) Collated dependences of the precession frequency $f_2$ on the fluence (circles), and of the qFMR frequency on the temperature $T_{\mathrm{BLS}}$ obtained from BLS data (stars).

We ascribe it to the fact that, at $T_0$ being in a vicinity of $T_{\mathrm{SR}}$, the excited system returns to different initial states after each pump pulse. Then the system is excited to a distinct state by a subsequent pulse. This is due to the fact that the first-order phase transitions are characterized by a sharp change in the thermodynamic properties of the system when passing through the transition temperature, where stability of the system is lost and fluctuations increase greatly. Thus, the closer the initial temperature of the sample is to the transition, the greater is the contribution to the transition from increasing fluctuations, as see at $T_0 \backsim T_{\mathrm{SR}}$ [see the data at $T_0 = 396$ K in Fig. 4(a)].

In addition, the magneto-optical pump-probe signal at a fixed fluence $F = 0.35$ J/cm$^2$ for various initial temperature [Fig. 4(g)] and at fixed temperature $T_0 = 365$ K for various fluence [Fig. 5(a)] was measured.

For characterizing the magnetic state at latency $\tau_{\mathrm{L}}$ and final time $t > 100$ ps, we obtained values of $\Delta\theta_{\mathrm{L}}$ and $\Delta\theta_{\mathrm{F}}$ as shown in Fig. 4(b, h) and Fig. 5(b). Using these values and Eq.(1) from the main text, we calculated the magnetization mismatch parameter $\Delta_{\mathrm{M}}$ [Fig.4(c, i)

and Fig. 5(c)] and the switched fraction $N^{\mathrm{SW}}$ [Fig. 4(d, j) and Fig. 5(c)]. The latency $\tau_{\mathrm{T}}$ was obtained as described in Sec. IX [Fig. 4(e, k) and Fig. 5(e)]. The precession frequency during the SR transition is used for finding the final temperature $T_{\mathrm{F}}$ by collating two dependence: the laser-induced precession frequency $f_2$ and the equilibrium qFMR frequency obtained from BLS as illustrated in Fig. 4(f, l) and Fig. 4(f).

## VI. BRILLOUIN LIGHT SCATTERING

The quasi-ferromagnetic resonance mode (qFMR) was studied using the Brillouin light scattering (BLS) technique in the back scattering geometry. A single-mode laser with a wavelength of 532 nm is focused on the sample surface into a spot with a diameter of 25 μm using an objective lens. Frequency resolution is achieved using a Fabry-Perot interferometer. All experiments are carried out at $T_0 = 418 - 465$ K in an external magnetic field of $\mu_0 H$ = 200 mT applied in the sample plane along the $c$-axis.

Fig. 6 shows the BLS spectra obtained at various temperatures, their fit using Gaussian function, and the extracted qFMR frequencies.

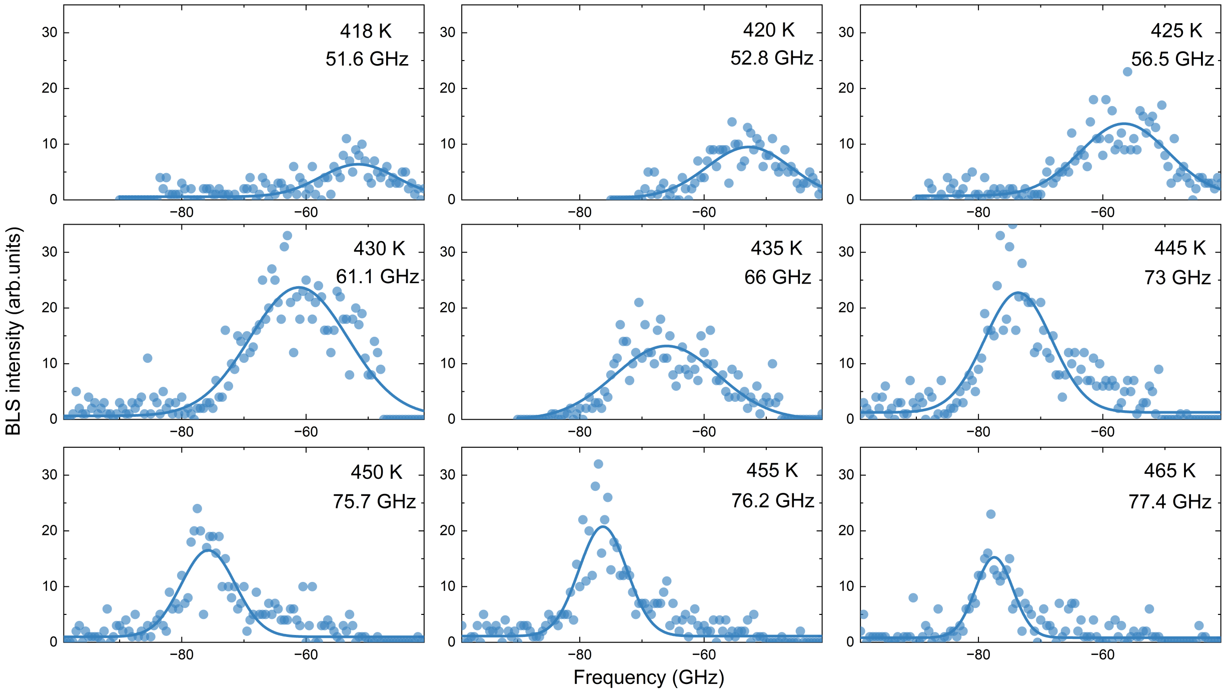


FIG. 6. BLS spectrum of $Fe_3BO_6$ at $\mu_0 H$ =200 mT and various temperatures. Solid lines are Gauss fits.

## VII. CALCULATION OF THE LASER-INDUCED HEATING

Temperature increase $\Delta T$ and the resulting temperature $T_\mathrm{h} = T_0 + \Delta T$ are calculated as a function of the pump fluence $F$ (at $T_0 = 385$ K) and of the initial temperature $T_0$ (at $F$=0.5 J/cm$^2$). For calculations, volumetric absorbed pump energy density $J$ is found from the incident fluence as

$$J = (1 - R)\alpha F, \tag{7}$$

where $R = 0.38$ is a reflection coefficient [6], and $\alpha = 4.5{\cdot}10^5$ cm$^{-1}$ is the absorption coefficient [7] of $Fe_3BO_6$ at the experimental pump wavelength. The temperature increase is calculated as

$$T_\mathrm{h} = T_0 + \frac{J}{C_\mathrm{V}}, \tag{8}$$

where $C_\mathrm{V} = C \cdot \rho = 4.3 \cdot 10^6$ J$\cdot$(m$^3$ K)$^{-1}$ is a volumetric heat capacity. To calculate these values, we use density of the iron borate $\rho$ =4760 kg$\cdot$m$^{-3}$ [8] and heat capacity $C$ =900 J$\cdot$(kg$\cdot$K)$^{-1}$ of the hematite [9] at $T_0 = 385$ K, since the heat capacity of the iron borate is not available in the literature. Using the dependence of the volumetric heat capacity on temperature, the heating of $Fe_3BO_6$ is also calculated for different temperatures $T_0$ at the fixed pump fluence $F = 0.5$ J/cm$^2$. The resulting $T_\mathrm{h}$ [Fig. 7] are close to the temperatures estimated based on the precession frequency, as described in the main text.

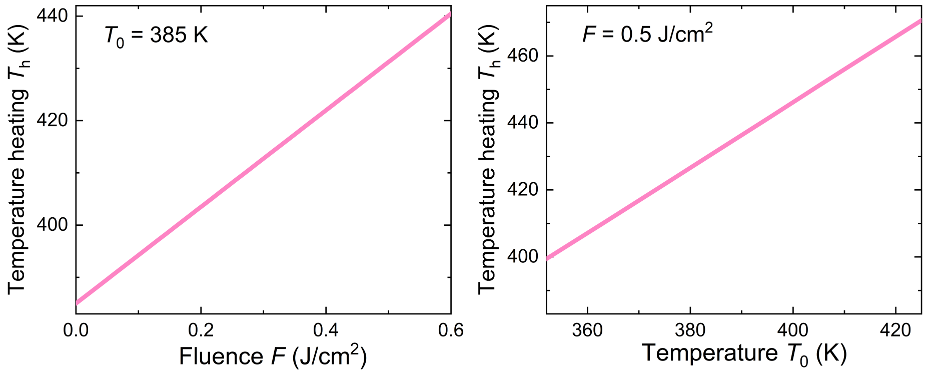


FIG. 7. Laser-induced heating $T_\mathrm{h}$ as a function of (a) the pump fluence at fixed initial temperature $T_0 = 385$ K and (b) the initial temperature $T_0$ at fixed pump fluence $F = 0.5$ J$\cdot$cm$^{-2}$.

## VIII. LASER-INDUCED REFLECTIVITY CHANGE

To confirm that the evolution of $\Delta\theta(t)$ at $t < t_{\mathrm{SR}}$ does not correlate with the transient optical properties, we measured laser-induced reflectivity change. The intensity change $\Delta R(t)$ of the reflected probe pulse was measured as a function of the delay time between the pump and probe pulses using a balanced photodetection scheme with a reference beam split from the incident probe beam. For this, the experimental setup was modified as illustrated in Fig. 8(b).

We investigated the transient reflectivity change upon excitation by pump pulses with different polarization angles [Fig. 8(a)] and compared with the transient Kerr rotation $\Delta\theta(t)$ [Fig. 8(c)] obtained under the same conditions. From comparison of the two sets of time traces it is evident that at the time range of latency $\tau_{\mathrm{L}}$ (shadowed range) the optical reflectivity does not contain peculiarities as those observed in the Kerr rotation $\Delta\theta$. Furthermore, pump fluence dependence of $\Delta R$, as well as its temperature dependence are linear [Figs. 8(e,f)], in contrast to the corresponding dependences of $\Delta\theta_{\mathrm{L}}$ [Figs. 3(b) and 4(b) in the main text]. This observations confirms that the transient Kerr signal at $t < t_{\mathrm{SR}}$ originates from evolution of the magnetic state and not from reflectivity change.

One notes that the change of the pump polarization affects both $\Delta R$ and $\Delta\theta$ transients. The change of the transient Kerr rotation with the pump polarization is similar to the change due to the variation of the pump fluence [Fig. 3(a) in main Letter]. The reflectivity magnitude varies with the pump polarization angle as shown in Fig. 8(d). We ascribe the observed dependences on the pump polarization to the anisotropy of the absorption coefficient of $Fe_3BO_6$ [10].

Finally, we address the origin of the oscillations present in the $\Delta R(t)$ signals. Their frequency is $\approx$ 80 GHz and is independent of the initial temperature and the fluence, as shown in the Fig. 8(e,f). Based on these observations, we conclude that these are Brillouin oscillations due to acoustic phonon generated through the thermoelastic effect as routinely observed in such experiments due to femtosecond laser pulse absorption [11].

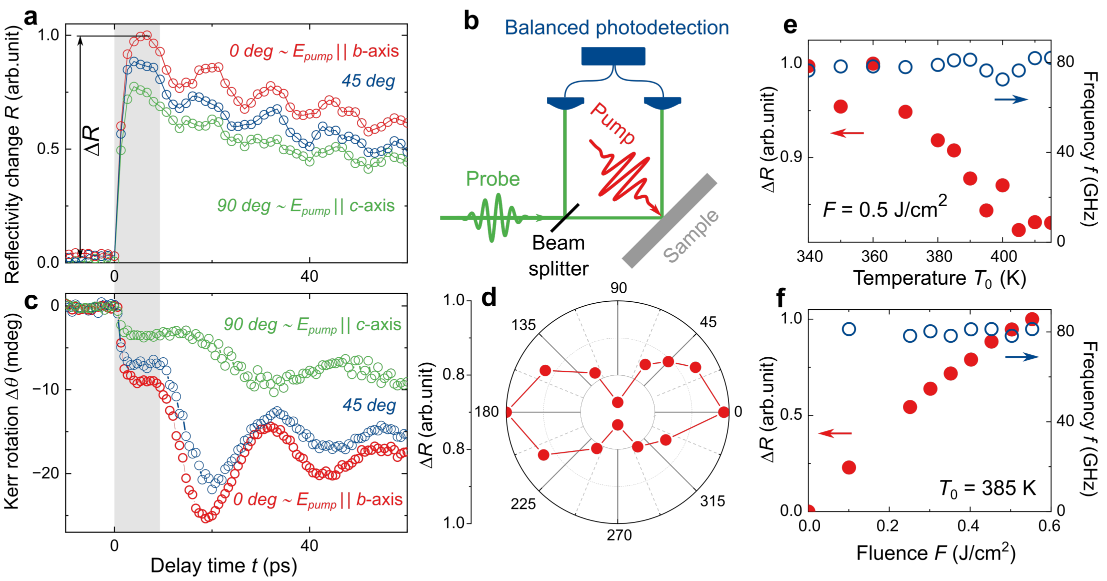


FIG. 8. (a) Reflectivity change $R$ and (c) polarization rotation $\Delta\theta$ measured at $T_0$= 385 K and $F = 0.5$ J/cm$^2$ as a functions of the delay time $t$ between pump and probe pulses at difference pump polarization. (b) Scheme of measuring laser-induced reflectivity change by balanced photodetection. Laser-induced reflectivity change $\Delta R$ as a function of (d) the pump polarization, (e) the initial temperature and (f) the fluence. In addition, in the panels (e, f) frequency of Brillouin oscillations is shown.

## IX. LATENCY

The latency $\tau_{\mathrm{L}}$ is defined as the time range during which the signal $\Delta\theta(t)$ does not change. To determine $\tau_{\mathrm{L}}$, the time derivatives of the signals and of their fits [Eq. 2], $d(\Delta\theta)/dt$, were obtained. In Fig. 9 (a-c) the derivatives are shown as obtained from the data under various fluences, initial temperatures, and applied fields. The latency $\tau_{\mathrm{T}}$ depends on the pump fluence [Fig. 3(e) in the main manuscript], the initial temperature of the sample [Fig. 4(e)] and the magnetic field [Fig. 9(d)].


[1] R. Wolfe, R. D. Pierce, M. Eibschütz, and J. W. Nielsen, Magnetization and mössbauer effect in single crystal $Fe_3BO_6$, Solid State Communications **7**, 949 (1969).

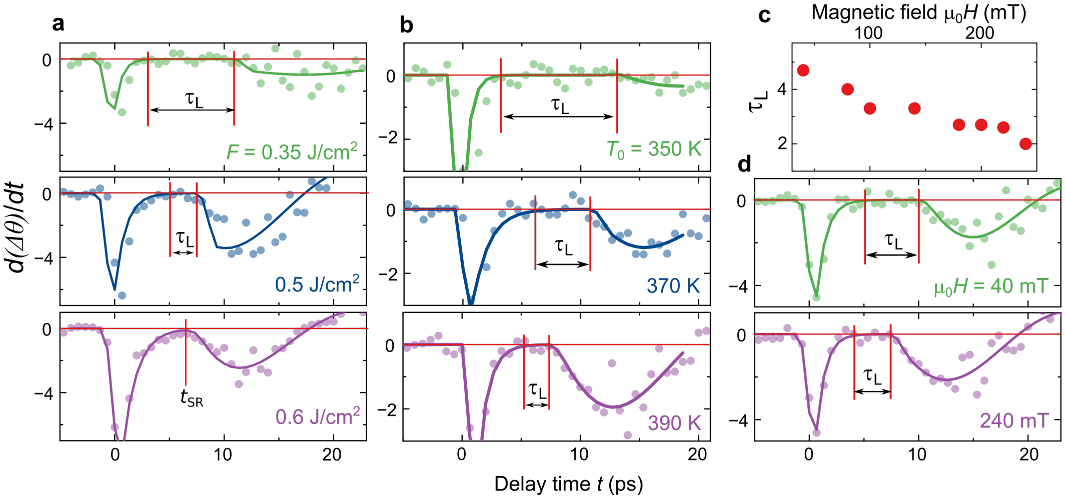


FIG. 9. Derivatives of the experimental signals (symbols) and of theirs fits (lines) at $\mu_0 H$ =200 mT and (a) various laser fluences at the fixed $T_0$ = 385 K, and (b) various initial temperatures at the fixed $F$ = 0.5 J·cm$^{-2}$. (c) Magnetic field dependence of the latency $\tau_L$ obtained from the data and their fits measured at different fields at fixed $F$ = 0.5 J·cm$^{-2}$ and $T_0$ = 385 K [panel (d)].


[2] V. I. Ozhogin, V. G. Shapiro, K. G. Gurtovoi, E. A. Galst'yan, and A. Y. Chervonenkis, Statics and linear dynamics of orthoferrites-phase transition of the "one-and-one-half"th kind, Soviet Physics JETP **35**, 1162 (1972).

[3] K. P. Belov, A. K. Zvezdin, A. M. Kadomtseva, and R. Z. Levitin, Spin-reorientation transitions in rare-earth magnets, Soviet Physics Uspekhi **19**, 574 (1976).

[4] A. G. Gurevich and G. A. Melkov, Magnetization oscillations and waves (CRC press, 2020).

[5] V. E. Arutyunyan, K. N. Kocharyan, and R. M. Martirosyan, Magnetic resonance in the orthorhombic antiferromagnet $Fe_3BO_6$, Soviet Physics JETP **69**, 783 (1989).

[6] M. Abe, H. Nakagawa, M. Gomi, and S. Nomura, A reflection method of determining birefringence and refractive index in orthorhombic crystal, Japanese Journal of Applied Physics **19**, 1077 (1980).

[7] B. Andlauer, R. Diehl, and M. S. Skolnick, Investigation of the optical absorption of $Fe_3BO_6$ after oxygen annealing and under the influence of strong magnetic fields, Journal of Applied Physics **49**, 2200 (1978).

[8] R. Diehl and G. Brandt, Refinement of the crystal structure of $Fe_3BO_6$, Acta Crystallographica B **31**, 1662 (1975).

[9] F. Grønvold and A. Sveen, Heat capacity and thermodynamic properties of synthetic magnetite ($Fe_3O_4$) from 300 to 1050 K. ferrimagnetic transition and zero-point entropy, The Journal of Chemical Thermodynamics **6**, 859 (1974).

[10] B. Andlauer and R. Diehl, Optical absorption of $Fe_3BO_6$ in the range of the transitions $^6A_1 \rightarrow {}^4T_1$, $^4T_2$, Physica B+C **89**, 50 (1977).

[11] O. Matsuda, M. C. Larciprete, R. Li Voti, and O. B. Wright, Fundamentals of picosecond laser ultrasonics, Ultrasonics **56**, 3 (2015).
